# Supplementary material for: Tunable topology, Hall response, and spin-textures in bicircularly polarized light illuminated altermagnets
Source: arXiv:2509.06349 source file (2025-09-08)
Supplement: Supplementary file 1 [file supple_light_on_altermagnet.pdf]

Supplemental Material for “Tunable topology, Hall response, and  
spin-textures in bicircularly polarized light illuminated  
altermagnets”

This Supplemental Material includes the details of derivation of the Floquet effective Hamiltonian, plots of band structures, discussion on controlling symmetry of the model using BCL, and tunable spin texture plots.

## S1. DERIVATION OF THE FLOQUET EFFECTIVE HAMILTONIAN

After Peierls substitution, the tight-binding Hamiltonian for the  $d_{x^2-y^2}$ -wave altermagnet with RSOC takes the form,

$$\begin{aligned}
H(\mathbf{k}, t) = & -2t_t(\cos k_x \cos A_x(t) - \sin k_x \sin A_x(t) + \cos k_y \cos A_y(t) - \sin k_y \sin A_y(t))I - \mu I \\
& + 2t_j(\cos k_y \cos A_y(t) - \sin k_y \sin A_y(t) - \cos k_x \cos A_x(t) + \sin k_x \sin A_x(t))\sigma_z \\
& + 2\lambda(\sin k_y \cos A_y(t) + \cos k_y \sin A_y(t))\sigma_x - 2\lambda(\sin k_x \cos A_x(t) + \cos k_x \sin A_x(t))\sigma_y.
\end{aligned} \tag{1}$$

Therefore, the Fourier modes of the Hamiltonian can be expressed as,

$$\begin{aligned}
H_m(\mathbf{k}) = & -2t_t(\cos k_x f_m^{cx} - \sin k_x f_m^{sx} + \cos k_y f_m^{cy} - \sin k_y f_m^{sy} - \mu)I \\
& + 2t_j(\cos k_y f_m^{cy} - \sin k_y f_m^{sy} - \cos k_x f_m^{cx} + \sin k_x f_m^{sx})\sigma_z \\
& + 2\lambda(\sin k_y f_m^{cy} + \cos k_y f_m^{sy})\sigma_x - 2\lambda(\sin k_x f_m^{cx} + \cos k_x f_m^{sx})\sigma_y \\
= & d_m^0(\mathbf{k})I + d_m^x(\mathbf{k})\sigma_x + d_m^y(\mathbf{k})\sigma_y + d_m^z(\mathbf{k})\sigma_z \\
= & d_m^0(\mathbf{k})I + \mathbf{d}_m(\mathbf{k}) \cdot \boldsymbol{\sigma},
\end{aligned} \tag{2}$$

where,

$$\begin{aligned}
f_m^{ci} = & \frac{\omega}{2\pi} \int_0^{\frac{2\pi}{\omega}} \cos(A_i(t)) e^{-im\omega t} dt, \\
f_m^{si} = & \frac{\omega}{2\pi} \int_0^{\frac{2\pi}{\omega}} \sin(A_i(t)) e^{-im\omega t} dt ; i \in \{x, y\}.
\end{aligned} \tag{3}$$

We can see that  $\mathbf{d}_{-m}(\mathbf{k}) = \mathbf{d}_m(\mathbf{k})^*$ . Using the identity  $[\mathbf{a} \cdot \boldsymbol{\sigma}, \mathbf{b} \cdot \boldsymbol{\sigma}] = 2i(\mathbf{a} \times \mathbf{b}) \cdot \boldsymbol{\sigma}$ , we have

$$\begin{aligned}
[H_{+m}(\mathbf{k}), H_{-m}(\mathbf{k})] = & 2i(\mathbf{d}_m(\mathbf{k}) \times \mathbf{d}_m(\mathbf{k})^*) \cdot \boldsymbol{\sigma} \\
= & -2 \text{Im}(\mathbf{d}_m(\mathbf{k}) \times \mathbf{d}_m(\mathbf{k})^*) \cdot \boldsymbol{\sigma},
\end{aligned} \tag{4}$$

and

$$\begin{aligned}
& [H_0(\mathbf{k}), H_{+m}(\mathbf{k})] - [H_0(\mathbf{k}), H_{-m}(\mathbf{k})] \\
&= 2i(\mathbf{d}_0(\mathbf{k}) \times \mathbf{d}_m(\mathbf{k})) \cdot \boldsymbol{\sigma} - 2i(\mathbf{d}_0(\mathbf{k}) \times \mathbf{d}_m(\mathbf{k})^*) \cdot \boldsymbol{\sigma} \\
&= -4 \text{Im}(\mathbf{d}_0(\mathbf{k}) \times \mathbf{d}_m(\mathbf{k})) \cdot \boldsymbol{\sigma}.
\end{aligned} \tag{5}$$

In our numerical implementation, we have calculated the  $f$ -coefficients in Eq. 3 numerically for various light parameters and then have applied Floquet theory to determine the effective photon-dressed Hamiltonian.

## S2. CONTROLLING BAND-STRUCTURE AND CHERN NUMBER USING BCL

Here we illustrate, by showing the band structures of the altermagnets, that by changing the relative amplitude parameter,  $r$ , in BCL, it is possible to drive the system through a band-touching point even in the presence of non-zero illumination.

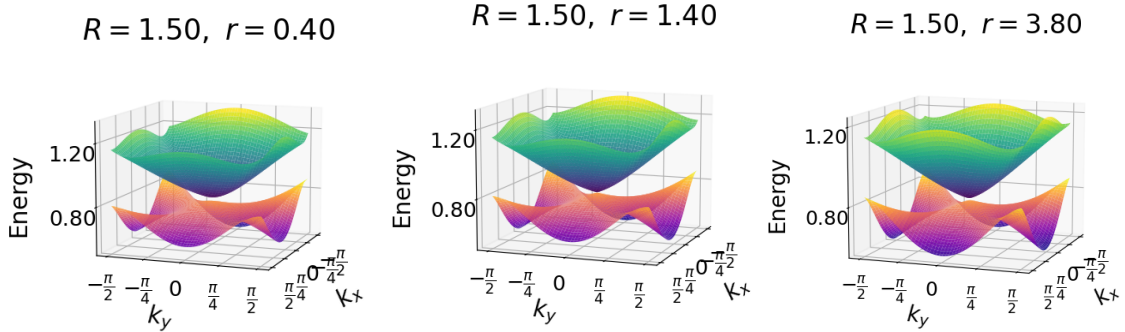

FIG. S1. **Dependence of the band-gap of  $d_{x^2-y^2}$ -wave altermagnet on relative amplitude  $r$ .** The plots show that the gap closes around  $r \approx 1.4$  for  $R = 1.50$ . Other chosen parameters are  $t_t = 0.1, t_j = 0.3, \lambda = 0.1, \mu = -1, \omega = 3, \alpha = 0$ , as from the Chern number plot. A gap opens up on further increase of  $r$ .

We also show the Chern number density plots in the overall amplitude ( $R$ )-relative amplitude ( $r$ )-plane for different strengths of the Rashba spin orbit coupling  $\lambda$  for fixed altermagnetic exchange coupling  $t_j$ , in Fig. S3 for  $d_{x^2-y^2}$ -wave altermagnet and in Fig. S4 for  $d_{xy}$ -wave altermagnet.

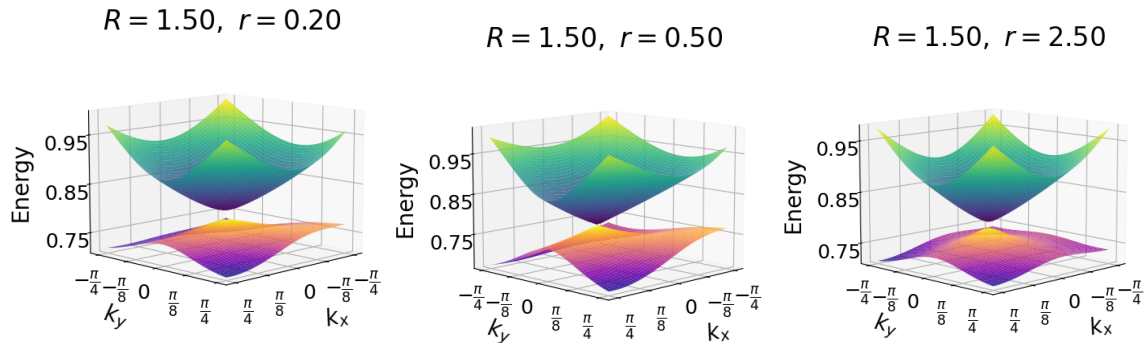

FIG. S2. **Dependence of the band-gap of  $d_{xy}$ -wave altermagnet on relative amplitude  $r$ .** The plots show that the gap closes around  $r \approx 0.5$  for  $R = 1.50$ . Other chosen parameters are  $t_t = 0.1, t_j = 0.3, \lambda = 0.1, \mu = -1, \omega = 3, \alpha = 0$ , as from the Chern number plot. A gap opens up on further increase of  $r$ .

### S3. CONTROLLING SYMMETRY OF THE MODEL USING BCL

In Floquet theory, the first term of the Floquet effective Hamiltonian  $H_F(\mathbf{k})$  is  $H_0(\mathbf{k}) = \overline{H(\mathbf{k}, t)} = T^{-1} \int_0^T H(\mathbf{k}, t) dt$  where  $T$  is the time-period. The subleading term is proportional to  $\omega^{-1}$  where  $\omega = 2\pi T^{-1}$ . Therefore, in the  $\omega \rightarrow \infty$  limit  $H_F(\mathbf{k}) = H_0(\mathbf{k})$ . For finite (but large)  $\omega$  the  $\omega^{-1}$  correction can be considered as a perturbation to  $H_0(\mathbf{k})$ . Therefore, understanding how  $H_0(\mathbf{k})$  differs from the actual  $H(\mathbf{k})$  will allow us to understand what *overall* changes are induced in the system as a result of light irradiation. Curiously,  $H_0(\mathbf{k})$  *does not depend on  $\omega$*  and can be computed by setting  $\omega = 1$  for convenience. We show this below (for clarification, showing explicit  $\omega$  dependence on the time-periodic Hamiltonian),

$$\begin{aligned}
 H_0(\mathbf{k}) &= \frac{\omega}{2\pi} \int_0^{\frac{2\pi}{\omega}} H(\mathbf{k}, t, \omega) dt \\
 &= \frac{1}{2\pi} \int_0^{2\pi} H\left(\mathbf{k}, \frac{t}{\omega}, \omega\right) dt \\
 &= \frac{1}{2\pi} \int_0^{2\pi} H(\mathbf{k}, t, \omega = 1) dt.
 \end{aligned} \tag{6}$$

Going to the second line, we performed a change of variable  $t \rightarrow \omega t$  and the last line follows from the fact that  $t$  always appears as a combination of  $\omega t$  in  $H(\mathbf{k}, t)$  after a Peierls substitution. This shows why  $H_0(\mathbf{k})$  does not depend on  $\omega$  (essentially, it can be rescaled away) and we can put  $\omega = 1$  for simplicity while calculating the time averages. As a matter of fact, it can be shown in a similar way that the higher harmonics  $H_m(\mathbf{k})$  also

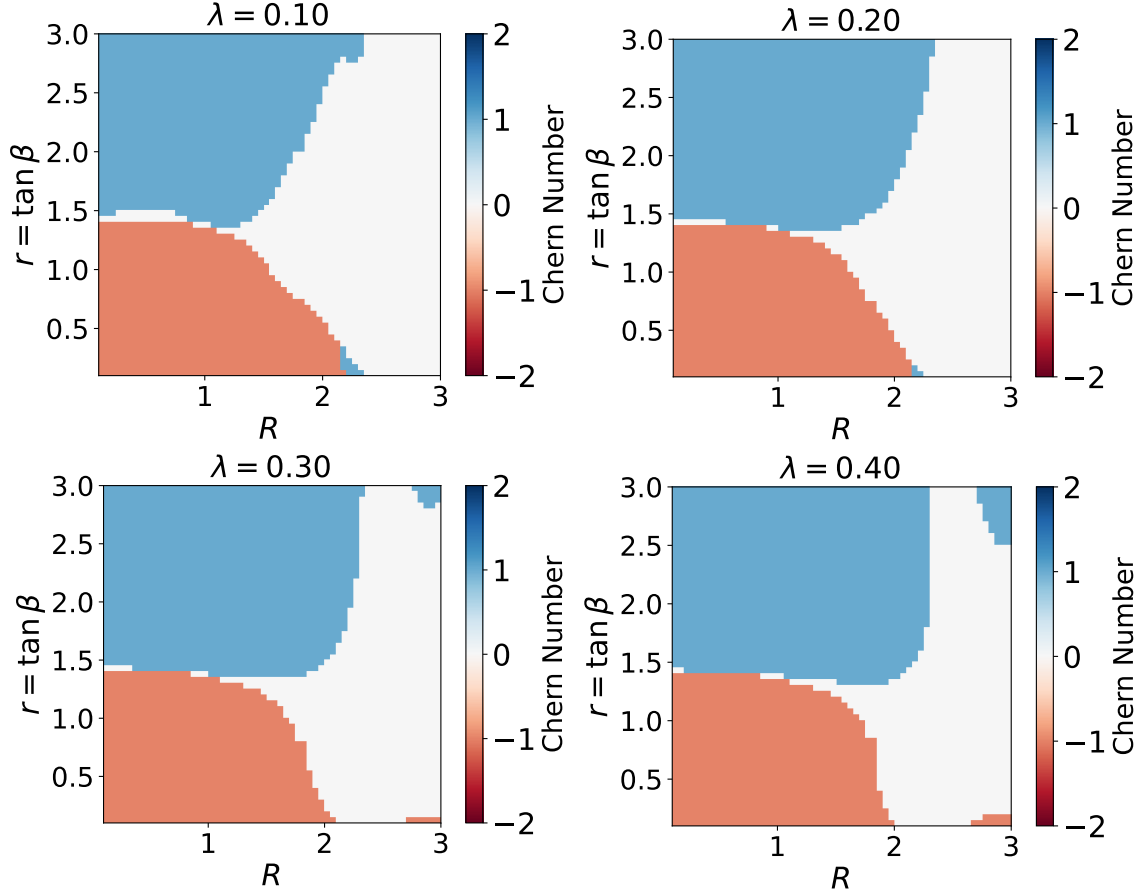

FIG. S3. **Chern number density plot for  $d_{x^2-y^2}$ -wave altermagnet.** Chosen parameters are  $t = 0.1, t_j = 0.3, \mu = -1, \omega = 3, \alpha = 0$ . The plots illustrate the dependence of Chern number on the Rashba spin orbit coupling  $\lambda$ .

do not depend explicitly on  $\omega$ . However, their relative importance in the Floquet effective Hamiltonian  $H_F(\mathbf{k})$  are dictated by the appearance of explicit  $\omega^{-k}$ ,  $k \in \mathbb{Z}^+$  factors in the Floquet-Magnus expansion. Let us next look at the two situations for the two types of altermagnets.

#### A. $d_{x^2-y^2}$ -wave altermagnet

The minimal model of a  $d_{x^2-y^2}$ -wave altermagnet with Rashba spin-orbit coupling that we consider is,

$$H(\mathbf{k}) = -2t(\cos k_x + \cos k_y)I + 2t_j(\cos k_y - \cos k_x)\sigma_z + 2\lambda(\sin k_y\sigma_x - \sin k_x\sigma_y). \quad (7)$$

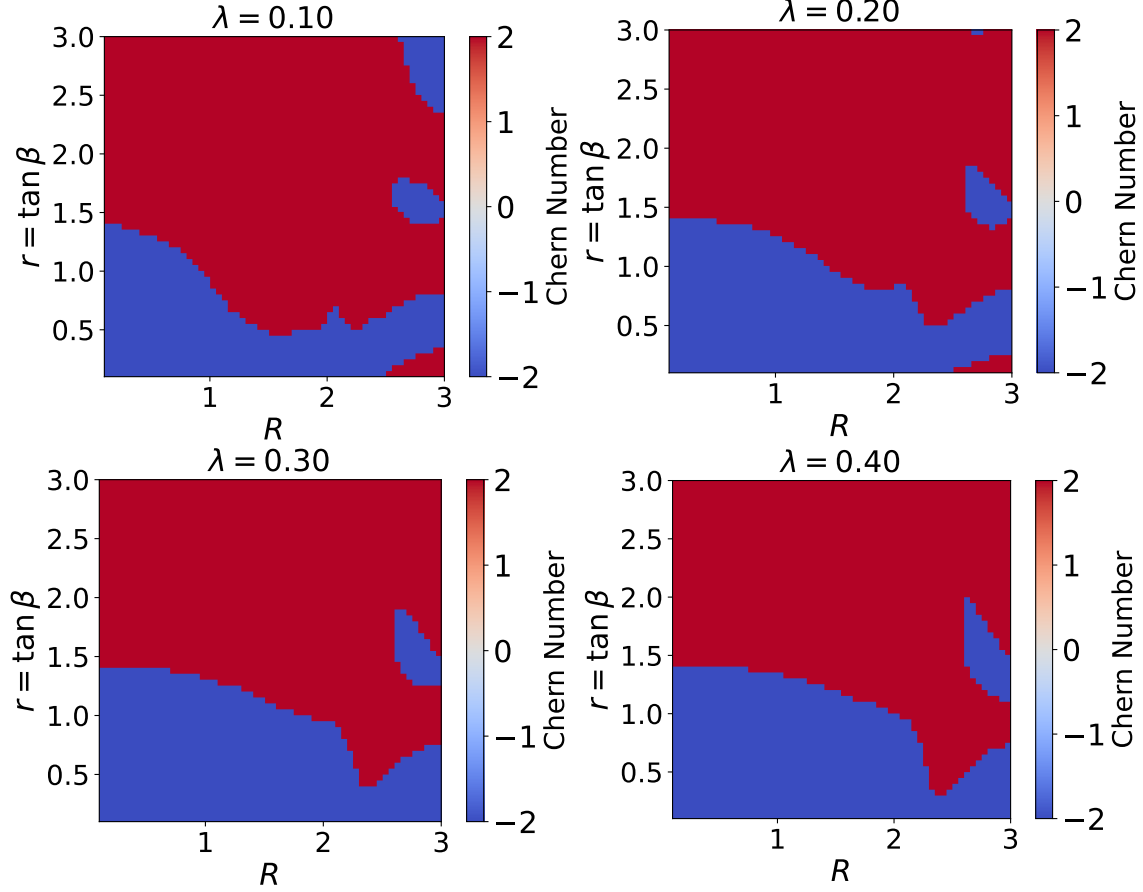

FIG. S4. **Chern number density plot for  $d_{xy}$ -wave altermagnet.** Chosen parameters are  $t = 0.1, t_j = 0.3, \mu = -1, \omega = 3, \alpha = 0$ . The plots illustrate the dependence of Chern number on the Rashba spin orbit coupling  $\lambda$ .

After Peierls substitution, we need to calculate  $H_0(\mathbf{k}) = \overline{H(\mathbf{k}, t)}$  for which need to evaluate terms of the form,

$$\begin{aligned}
 \overline{\cos(k_x + A_x)} &= \cos k_x \overline{\cos A_x} - \sin k_x \overline{\sin A_x} \\
 &= \cos k_x f_0^{cx} - \sin k_x f_0^{sx} \\
 &= \sqrt{(f_0^{cx})^2 + (f_0^{sx})^2} \cos(k_x + k_{0,x}), \quad \text{where, } \tan k_{0,x} = \frac{f_0^{sx}}{f_0^{cx}} \\
 &=: f_0^x \cos(k_x + k_{0,x}).
 \end{aligned} \tag{8}$$

Similarly, we have

$$\begin{aligned}
\overline{\sin(k_x + A_x)} &= f_0^x \sin(k_x + k_{0x}) \\
\overline{\sin(k_y + A_y)} &= f_0^y \sin(k_y + k_{0y}) \\
\overline{\cos(k_y + A_y)} &= f_0^y \cos(k_y + k_{0y}), \quad \text{where, } \tan k_{0y} = \frac{f_0^{sy}}{f_0^{cy}}.
\end{aligned} \tag{9}$$

Therefore, it is now apparent that the ‘center’ of the system is shifted to  $-\mathbf{k}_0$  where  $\mathbf{k}_0 = (k_{0x}, k_{0y})$ . Thus, it mimics the effect of a *static*  $U(1)$  *gauge field* and inversion symmetry about  $\mathbf{k} = 0$  is broken even in the presence of vanishing spin-orbit coupling. It is also equivalent to an effective *twisted boundary condition* in real space. Furthermore, all  $x$ -directional form factors (such as  $\sin k_x, \cos k_x$ ) attain a modulation  $f_0^x$  and  $y$ -directional form factors attain a modulation  $f_0^y$ . Before moving on to see what this shift  $-\mathbf{k}_0$  and form factor modulations are, we note an important point. If  $f_0^x = f_0^y$ , then  $R_{\pi/2}T$  symmetry remains intact, implying that  $H_0(\mathbf{k})$  still describes an altermagnet with a shifted BTP at  $\mathbf{k} = -\mathbf{k}_0$ . Instead, if  $f_0^x \neq f_0^y$  then  $R_{\pi/2}T$  symmetry is broken and  $H_0(\mathbf{k})$  no longer describes an altermagnet. Further, the bands gap out with a gap  $4t_j|f_0^x - f_0^y|$  at  $\mathbf{k} = -\mathbf{k}_0$  (the bands remain topologically trivial though). A non-zero RSOC  $\lambda$  is assumed to infer the previous statement. For  $\lambda = 0$ , the bands still touch each other along the lines described by the equation  $f_0^x \cos k_x - f_0^y \cos k_y = 0$ . It is also worthwhile to note that when  $R_{\pi/2}T$  is broken, the system acquires some net spin-polarization and, therefore, a magnetization (weak ferromagnetism). Next, we consider the two cases of CL and BCL.

**Circularly polarized light (CL).** As it turns out, for CL we always have  $\mathbf{k}_0 = (0, 0)$  and  $f_0^x = f_0^y$ . This implies that the altermagnetic symmetry  $R_{\pi/2}T$  remains intact in  $H_0(\mathbf{k})$ . The fact that the center never shifts can be proven by showing that  $f_0^{sx} = f_0^{sy} = 0$  for CL or elliptically polarized (EPL). In these cases, the generic form of a vector potential component is  $A_i = R_i \sin(\omega t - \alpha)$ . Therefore, it suffices to show that  $\overline{\sin A_i} = 0$ .

$$\begin{aligned}
\overline{\sin A_i} &= \frac{\omega}{2\pi} \int_0^{\frac{2\pi}{\omega}} \sin(R_i \sin(\omega t - \alpha)) dt = -\frac{1}{2\pi} \int_{-\pi-\alpha}^{\pi+\alpha} \sin(R_i \sin t') dt', \quad t' = \omega t - \pi - \alpha \\
&= 0.
\end{aligned} \tag{10}$$

This shows that  $f_0^{sx} = f_0^{sy} = 0$  for both CL and EPL. This further implies that  $f_0^x = |f_0^{cx}|$ ,  $f_0^y = |f_0^{cy}|$ . From the outset, it is clear that for EPL with  $R_x \neq R_y$ , we will generically have  $f_0^x \neq f_0^y$ , which breaks the altermagnetic symmetry. However, for a different kind of

EPL for which the major axis makes the same angle with both the  $x$  and  $y$ -axes (for which CL is a special case), taking  $A_x = R \cos(\omega t - \alpha_1)$  and  $A_y = R \sin(\omega t - \alpha_2)$ , it is possible (here  $A_x$  and  $A_y$  are just phase shifted, so that the integration of any function, here cosine, of these two variables are equal when the integration is over the full time period  $[0, 2\pi/\omega]$ ) to show that  $\overline{\cos A_x} = \overline{\cos A_y}$ . Therefore, in this case, altermagnetic symmetry is preserved. As a corollary of the above-mentioned results, we can deduce that for linearly polarized light (LPL) along some generic direction will break the altermagnetic symmetry unless it makes an equal angle ( $\pm\pi/4$ ) with the two axes.

***Bicircularly polarized light (BCL).*** We find that a generic BCL, or a bielliptically polarized light (BEL), will lead to  $\mathbf{k}_0 \neq 0$  as well as  $f_0^x \neq f_0^y$ , keeping aside some special configurations that we probe. The vector potential of BCL is,  $A_x = R_2 \cos(\eta\omega t - \alpha) + R_1 \cos(\omega t)$  and  $A_y = -R_2 \sin(\eta\omega t - \alpha) + R_1 \sin(\omega t)$ .

First of all, if  $\eta$  is odd then  $f_0^{sx} = f_0^{sy} = 0$ , leading to  $\mathbf{k}_0 = 0$ . This is because, in this case  $A_i$  contains only odd frequencies, and since the expansion of  $\sin A_i$  has only odd powers of  $A_i$  it is not possible to have any zero frequency or static component in  $\sin A_i$ . Therefore,  $\overline{\sin A_i} = 0$ . Furthermore, if only  $\eta = 4n + 3$ , for  $n \in \mathbb{Z}$ , then  $A_x$  and  $A_y$  are phase-shifted leading to  $f_0^x = f_0^y$ , which preserves altermagnetic symmetry. For  $\eta = 4n + 1$ , the altermagnetic symmetry will be broken.

In the even  $\eta$  case, we will have  $\mathbf{k}_0 \neq 0$  generically. Interestingly, the vector  $\mathbf{k}_0$  can be rotated in the Brillouin zone by changing the relative phase  $\alpha$ . Moving to altermagnetic symmetry, for generic values of  $\alpha$  we have  $f_0^x \neq f_0^y$ . For special values of the form  $\alpha = (2n + 1)\pi/4$  (that is,  $\alpha \bmod \pi/2 = \pi/4$ ), we have  $f_0^x = f_0^y$  that restores the altermagnetic symmetry. Curiously, for these special values of  $\alpha$ , the  $\mathbf{k}_0$  vector makes  $\pm\pi/4$  angle with the  $k_x, k_y$  axes meaning  $|k_{x0}| = |k_{y0}|$ . For  $\alpha \bmod \pi/2 = 0$  the modulations will be maximally anisotropic.

## B. $d_{xy}$ -wave altermagnet

The Hamiltonian of the  $d_{xy}$ -wave altermagnet can be written as,

$$\begin{aligned}
H(\mathbf{k}) &= -2t(\cos k_x + \cos k_y)I + 2t_j \sin k_x \sin k_y \sigma_z + 2\lambda(\sin k_y \sigma_x - \sin k_x \sigma_y) \\
&= -2t(\cos k_x + \cos k_y)I + 2\lambda(\sin k_y \sigma_x - \sin k_x \sigma_y) - t_j(\cos(k_x + k_y) - \cos(k_x - k_y))\sigma_z \\
&= H^I(\mathbf{k}) + H^{II}(\mathbf{k}).
\end{aligned} \tag{11}$$

Here  $H^I(\mathbf{k})$  is the part that arises from the nearest neighbor hopping, consisting of the identity part and the RSOC. On the other hand,  $H^{II}(\mathbf{k})$  consists of the next-to-nearest neighbor (or diagonal) hopping term which is the altermagnetic part. While  $H^I(\mathbf{k})$  enjoys time-reversal as well as the 4-fold rotational symmetry,  $H^{II}(\mathbf{k})$  is only invariant under the combination of the two. This gives rise to the spin-split band structure with zero net magnetization. Now, after the laser irradiation the time-averaged  $H_0(\mathbf{k})$  will have two contributions  $H_0^I(\mathbf{k})$  and  $H_0^{II}(\mathbf{k})$ . Discussion on  $H_0^I(\mathbf{k})$  will be qualitatively similar to that of a  $d_{x^2-y^2}$ -wave altermagnet. So, we focus on  $H_0^{II}(\mathbf{k})$  for the moment and make comparisons with  $H_0^I(\mathbf{k})$  when necessary to understand  $H_0(\mathbf{k})$ .

For notational simplicity, let us introduce the following,  $k_\pm = k_x \pm k_y$  and similarly  $A_\pm = A_x \pm A_y$ . Our purpose is to understand terms of the form  $\overline{\cos(k_\pm + A_\pm)} = f_0^\pm \cos(k_\pm + k_{0\pm})$ , where,

$$\begin{aligned}
f_0^\pm &= \sqrt{(f_0^{c\pm})^2 + (f_0^{s\pm})^2}, \quad f_0^{c\pm} = \overline{\cos A_\pm}, \quad f_0^{s\pm} = \overline{\sin A_\pm} \\
\tan k_{0\pm} &= \frac{f_0^{s\pm}}{f_0^{c\pm}}.
\end{aligned} \tag{12}$$

The shift components  $k_{0\pm}$  rotated to the original frame become,  $k'_{0x} = (k_+ + k_-)/2$ ,  $k'_{0y} = (k_+ - k_-)/2$ , with the shift vector  $\mathbf{k}'_0 = (k'_{0x}, k'_{0y})$ . The prime distinguishes the shift vector  $\mathbf{k}'_0$  in  $H_0^{II}(\mathbf{k})$  from the shift vector  $\mathbf{k}_0$  in  $H_0^I(\mathbf{k})$ . *We shall see that, generically, nearest-neighbor and next-to-nearest neighbor hopping terms experience different static gauge fields for BCL.*

We will infer some of the results by making an analogy with situation tackled in  $d_{x^2-y^2}$ -wave altermagnet with the correspondence  $k_+ \rightarrow k_x$ , and  $k_- \rightarrow k_y$ . Evidently, for the CL case, there will be no shift or unequal modulation for the form factors  $\cos k_+$  and  $\cos k_-$ . For EPL also there will be no shift,  $k_{0\pm} = 0$ , but there can be unequal modulations  $f_0^\pm$  depending on the orientation of the major axis of the EPL. For major axis orientation along  $\hat{\mathbf{x}}$  or  $\hat{\mathbf{y}}$ , we will have  $f_0^+ = f_0^-$ , and  $f_0^+ \neq f_0^-$  otherwise. Notably, this is opposite of what happens for modulations of form factors in  $H_0^I(\mathbf{k})$ . Therefore, with an EPL it is possible to

break  $R_{\pi/2}T$  in  $H_0^I(\mathbf{k})$ , keeping the same symmetry intact in  $H_0^{II}(\mathbf{k})$  or vice-versa. In any case,  $R_{\pi/2}$  is always broken in the full  $H_0(\mathbf{k})$  in the presence of EPL irradiation.

Now let us consider the analogy in case of BCL too. For the BCL vector potential discussed before,  $A_{\pm}$  turn out to be,

$$\begin{aligned} A_+ &= \sqrt{2}R_2 \cos(\eta\omega t - \alpha + \pi/4) + \sqrt{2}R_1 \cos(\omega t - \pi/4) \\ A_- &= \sqrt{2}R_2 \sin(\eta\omega t - \alpha + \pi/4) - \sqrt{2}R_1 \sin(\omega t - \pi/4). \end{aligned} \quad (13)$$

The terms are arranged in a way to make their analogy with the original  $A_x$  and  $A_y$  manifest. The final step to establish the analogy is to perform a time translation  $\omega t \rightarrow \omega t + \pi/4$ ,

$$\begin{aligned} A_+ &= \sqrt{2}R_2 \cos(\eta\omega t - \alpha') + \sqrt{2}R_1 \cos(\omega t) \\ A_- &= \sqrt{2}R_2 \sin(\eta\omega t - \alpha') - \sqrt{2}R_1 \sin(\omega t), \quad \alpha' = \alpha - (\eta + 1)\pi/4. \end{aligned} \quad (14)$$

Just to reiterate an already discussed result, for odd  $\eta$  there is no shift  $k_{0\pm} = 0$ , but there can be an anisotropy in the modulations depending on whether  $\eta \bmod 4 = 1$  or  $\eta \bmod 4 = 3$ . This will hold true for both  $H_0^{II}(\mathbf{k})$  and  $H_0^I(\mathbf{k})$  at once. The case becomes interesting when  $\eta$  is even. In that case,  $(\alpha \bmod \pi/2 = 0) \implies (\alpha' \bmod \pi/2 = \pi/4)$  and  $(\alpha \bmod \pi/2 = \pi/4) \implies (\alpha' \bmod \pi/2 = 0)$ . Therefore, the rotational properties of  $H_0^{II}(\mathbf{k})$  and  $H_0^I(\mathbf{k})$  are somewhat at tension. In the former case  $R_{\pi/2}$  is broken in  $H_0^I(\mathbf{k})$  but  $R_{\pi/2}T$  is preserved in  $H_0^{II}(\mathbf{k})$ , while in the latter case  $R_{\pi/2}$  is preserved in  $H_0^I(\mathbf{k})$ , but  $R_{\pi/2}T$  is broken in  $H_0^{II}(\mathbf{k})$ . In any case  $T$  is always preserved in  $H_0^I(\mathbf{k})$ . However, the shifts  $\mathbf{k}'_0$  and  $\mathbf{k}_0$  are approximately in agreement direction-wise.

#### S4. CONTROLLING SPIN-TEXTURE WITH BCL PARAMETER $\alpha$

We illustrate how the spin-texture can be controlled by tuning the BCL parameter  $\alpha$  for both  $d_{x^2-y^2}$ -wave and  $d_{xy}$ -wave altermagnets.

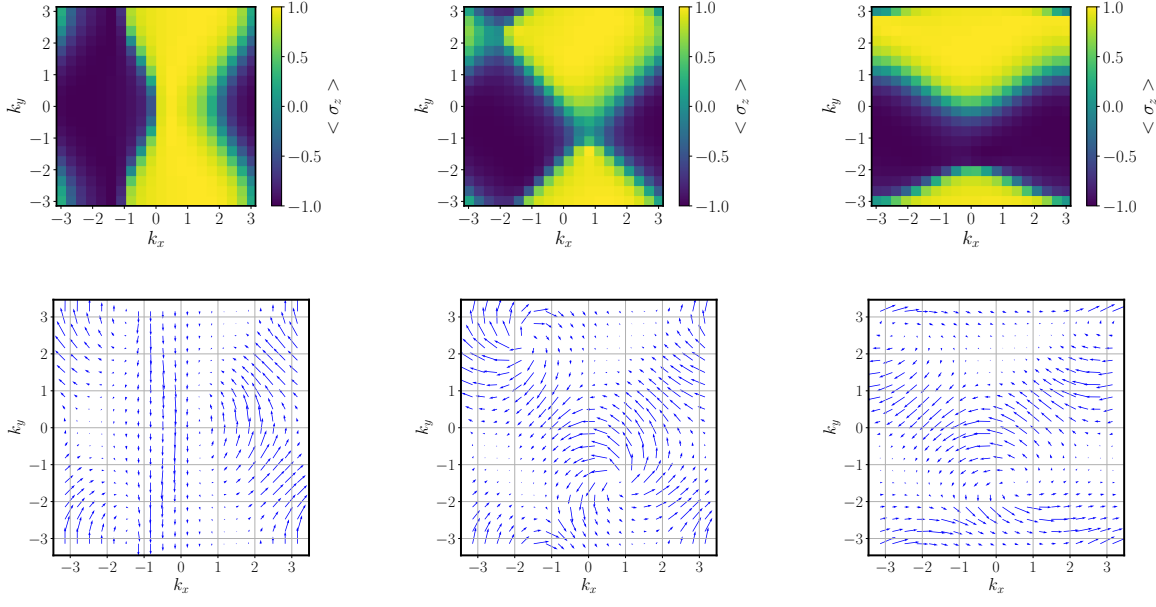

FIG. S5. **Spin-texture in  $d_{x^2-y^2}$ -wave altermagnet controlled by BCL.** The figures show how the spin structure of the effective Hamiltonian can be manipulated by changing the BCL parameter  $\alpha$ . The left column corresponds to  $\alpha = 0$  and the middle and right columns correspond to  $\alpha = \pi/4$  and  $\alpha = \pi/2$ , respectively. For these plots we have taken  $t_j = 0.3, \lambda = 0.1, \omega = 3, R = 2.2$  and  $r = 0.5$ . Note that the spin-texture does not depend on  $t$  or  $\mu$ .

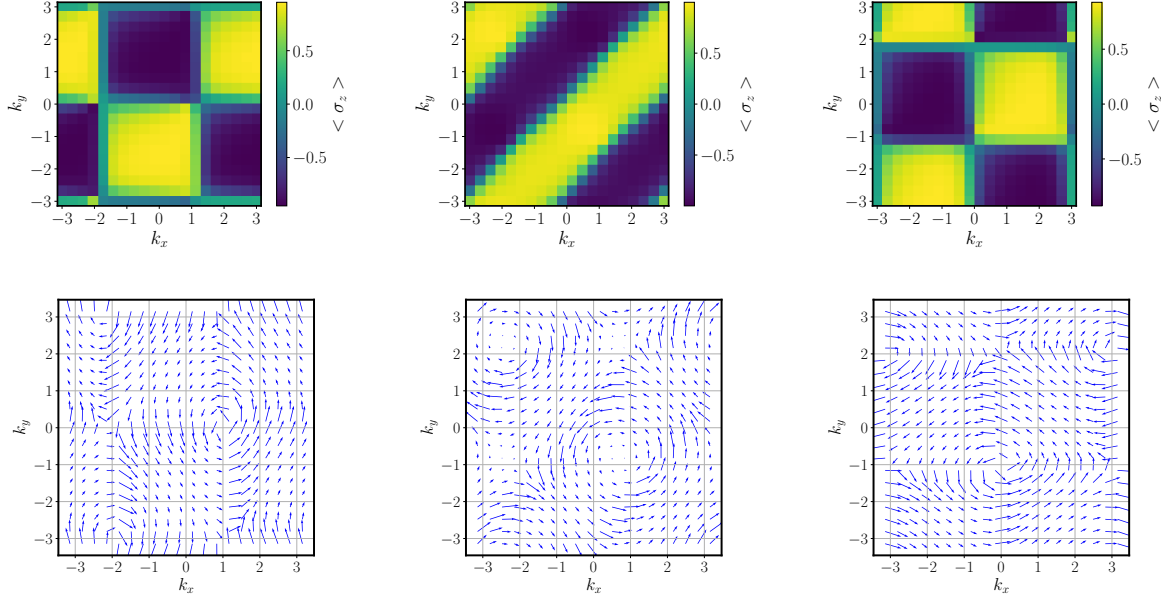

FIG. S6. **Spin-texture in  $d_{xy}$ -wave altermagnet controlled by BCL.** The figures show how the spin structure of the effective Hamiltonian can be manipulated by changing the BCL parameter  $\alpha$ . The left column corresponds to  $\alpha = 0$  and the middle and right columns correspond to  $\alpha = \pi/4$  and  $\alpha = \pi/2$ , respectively. For these plots we have taken  $t_j = 0.3, \lambda = 0.1, \omega = 3, R = 2.2$  and  $r = 0.5$ . Note that the spin-texture does not depend on  $t$  or  $\mu$ .
